# Supplementary material for: DiffMIC: Dual-Guidance Diffusion Network for Medical Image Classification
Source: arXiv:2303.10610 source file (2023-07-11)
Supplement: Supplementary file 1 [file supp.tex]

% This is samplepaper.tex, a sample chapter demonstrating the
% LLNCS macro package for Springer Computer Science proceedings;
% Version 2.20 of 2017/10/04
%
%\subsection{PMG2000}
%We collect and annotate a benchmark dataset (denoted as PMG2000) for placental maturity grading (PMG) with four categories, which is the largest public dataset for this task to our best knowledge.
%This dataset has 2098 B-mode ultrasound images captured by the vendors, \ie, GE Voluson E8 Expert and Phillip EPIQ7, including 518 images with Grade 0, 501 images with Grade I, 548 images with Grade II, and 531 images with Grade III.
\appendix
\section{Placental Maturity Grading}
\begin{table*}
\centering
\caption{\textbf{The details of our collected PMG2000.} To our best knowledge, this is the largest public dataset for the placental maturity grading task with four categories.}
\resizebox{1.0\textwidth}{!}{%
\begin{tabular}{c|c|c|c|c|c|c|c} 
\toprule
\multirow{2}{*}{\textbf{Dataset}} & \multirow{2}{*}{\textbf{Modality}} & \multirow{2}{*}{\textbf{Vendors}}     & \multicolumn{4}{c|}{\textbf{Grade}} & \multirow{2}{*}{\begin{tabular}[c]{@{}c@{}}\textbf{Total}\\\textbf{Num}\end{tabular}}  \\ 
\cline{4-7}
                                  &                                    &                                      & \textbf{0}   & \textbf{1}   & \textbf{2}   & \textbf{3}                 &                                   \\ 
\hline
PMG2000                           & B-mode ultrasound                  & GE
  Voluson E8 Expert/Phillip EPIQ7 & 518 & 501 & 548 & 531               & 2098                              \\
\bottomrule
\end{tabular}
}
\end{table*}

%
%All images are taken from the anterior wall placenta, and the subjects involved in PMG2000 are pregnant women aged from 18 to 40 weeks.
%
%All these placenta images are taken by ultrasound doctors with more than 5 years of clinical experience to ensure the image quality.
\begin{figure*}
\centering
\includegraphics[width=0.9\textwidth]{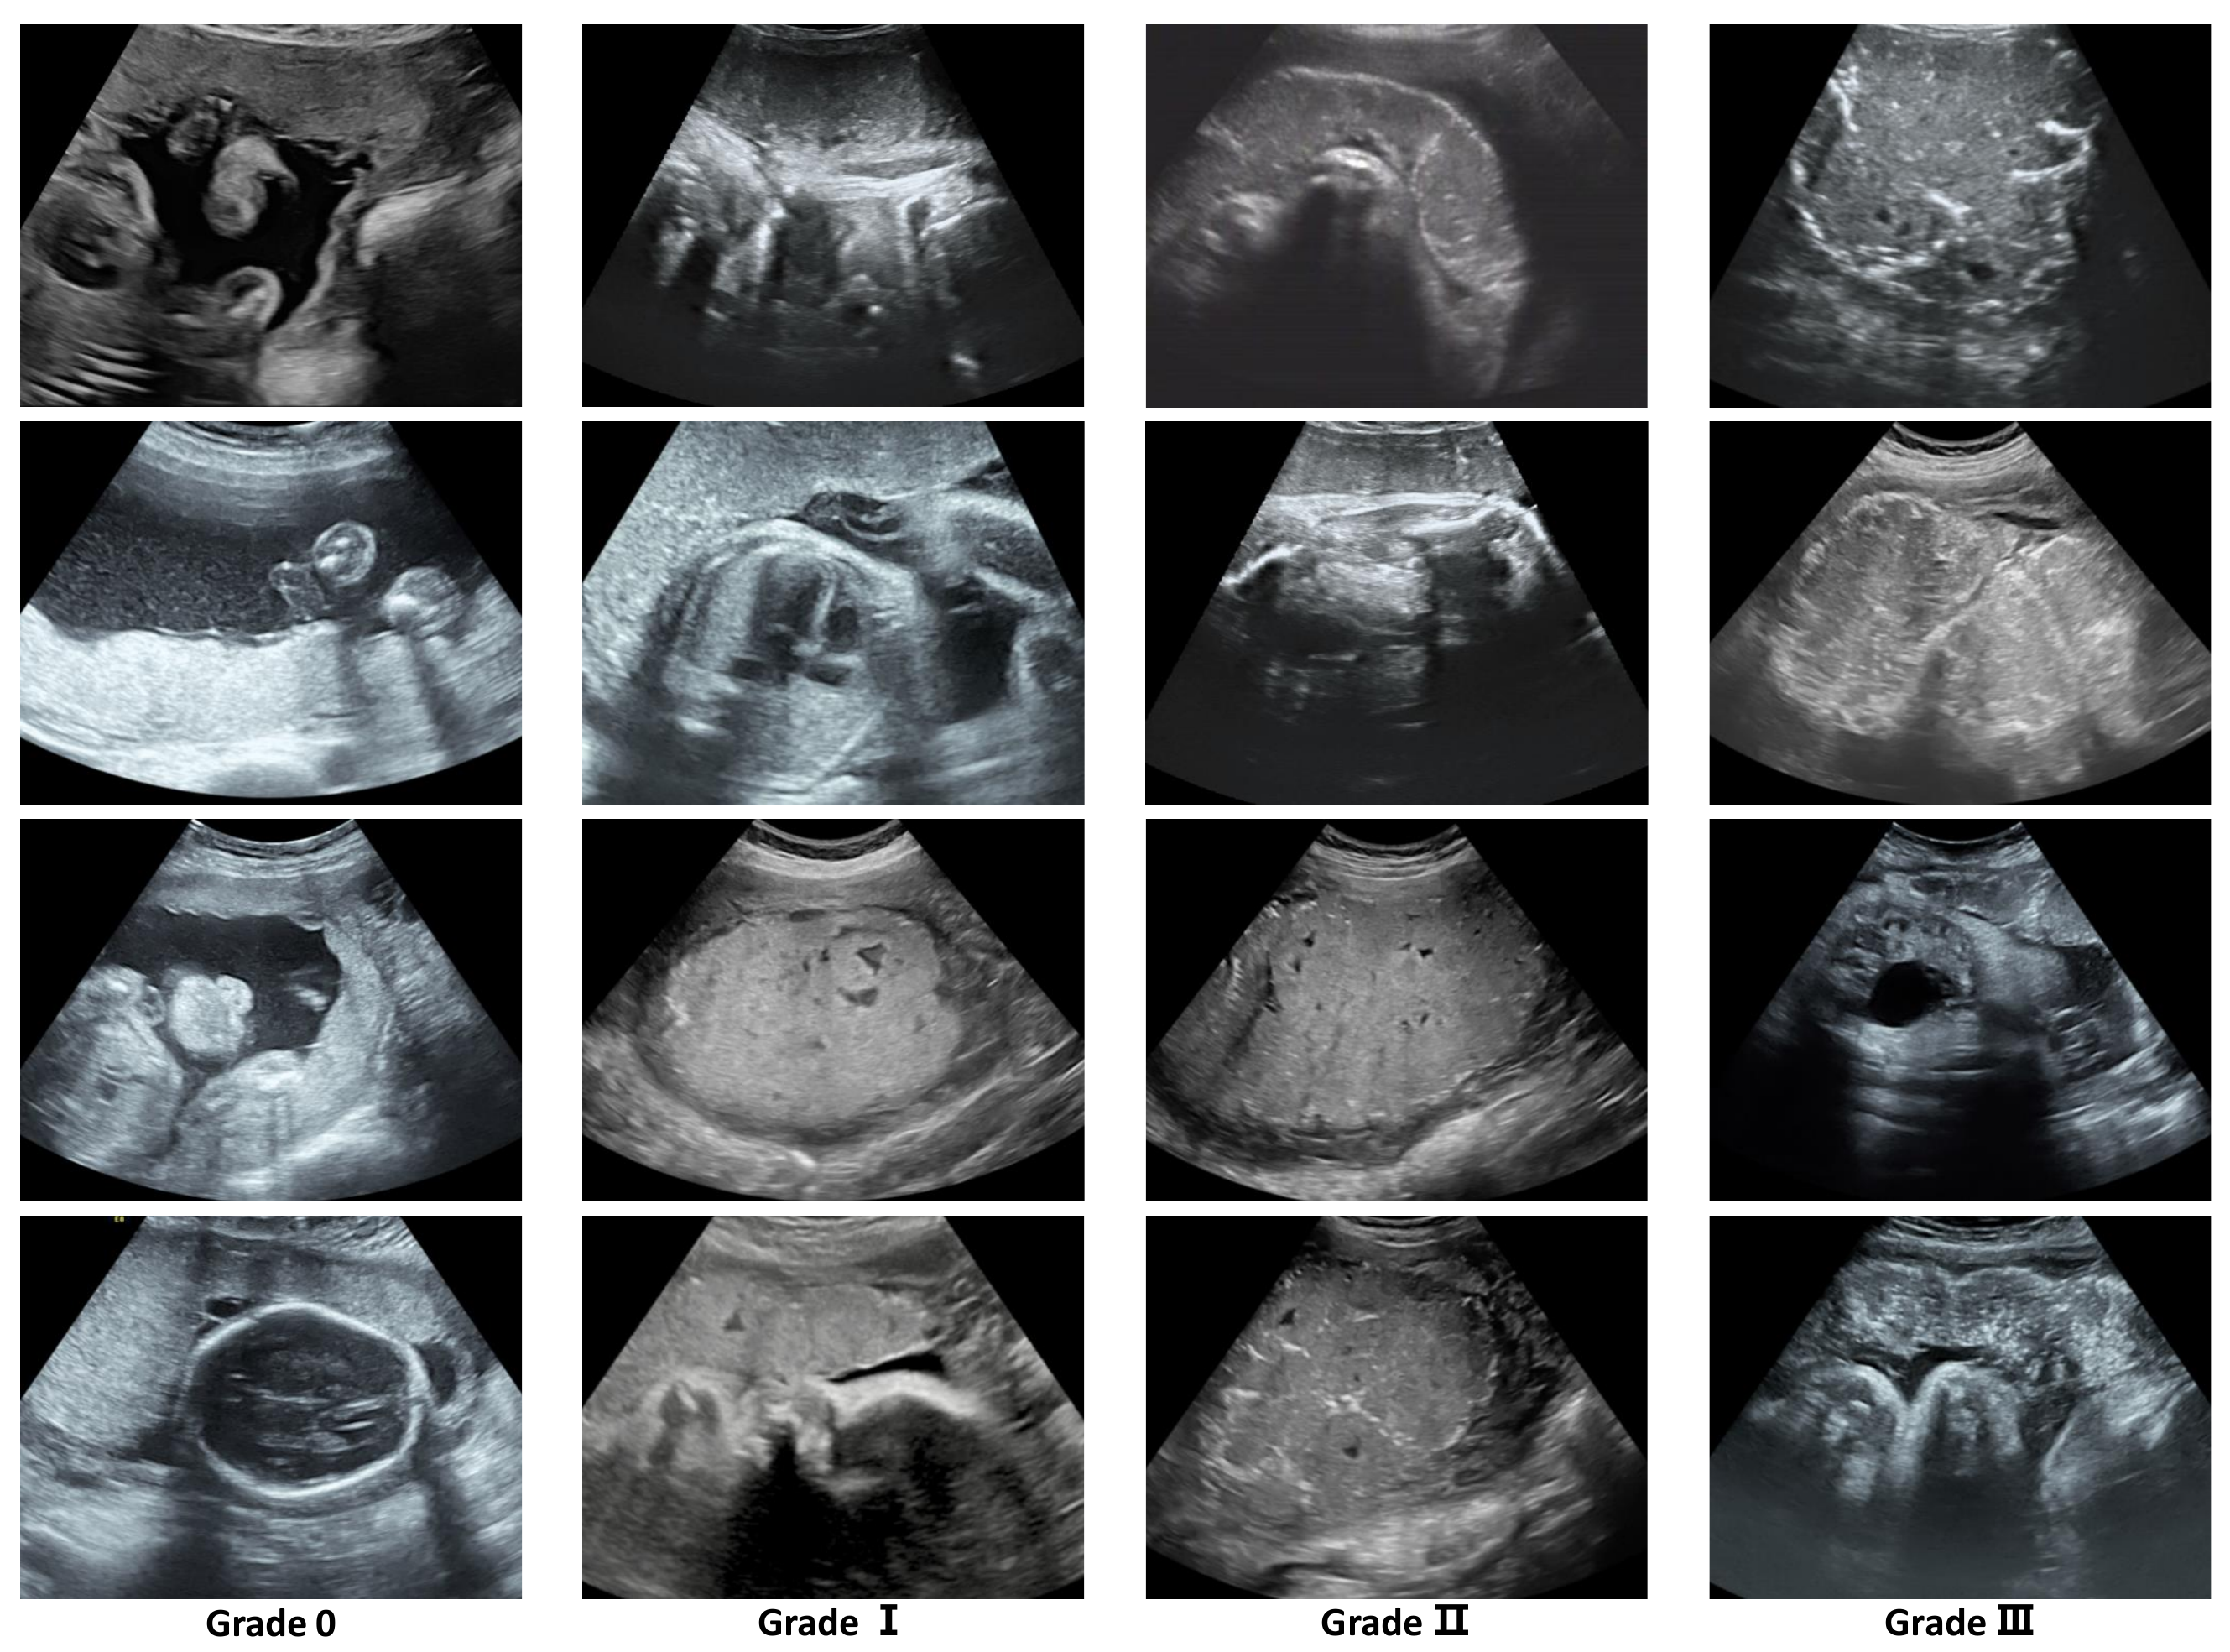}
\vspace{2pt}
\caption{\textbf{Several cases of four levels of placental maturity are presented.} All images are taken from the anterior wall placenta, and the subjects involved in PMG2000 are pregnant women aged from 18 to 40 weeks. They are taken by ultrasound doctors with more than 5 years of clinical experience to ensure the image quality.}\label{fig:example}
\end{figure*}
